# Supplementary material for: PVASS Reachability is Decidable
Source: arXiv:2504.05015 source file (2026-02-18)
Supplement: Supplementary file 1 [file appendix_ek_1.tex]

\newpage

Since all other 
However, it might be the case that even if 
Intuitively, an NGVAS is simply decomposable, if we can forget
Let $\simplydecomps$ be the set of labels that are simply decomposable.

\ek{Whenever choosing from $\concincount$, do not make $\adimset$ counters into $\omega$'s.}

\ek{What if $\concincount\cap\adimset=\emptyset$?}

\ek{Define $\compwith$}

\begin{proof}[Proof of \Cref{Lemma:SimplyDecomposable}]
    Let $\amarking, \amarkingp\in\Nomega^{d}$ and $\anonterm\in\nonterms$ with $\amarking\sqsubseteq\inof{\anonterm}$, $\amarkingp\sqsubseteq\outof{\anonterm}$, and $\omegaincount\subseteq\omegaof{\amarking}$.
    Further let $\amarking_{\omega}=\settoomega{\omegaincount\cup\set{i}}{\amarking}$, and $\amarkingp_{\omega}=\settoomega{\omegaoutcount\cup\set{j}}{\amarkingp}$ for $i,j\in\concincount\cap\adimset$.
    Assume that $\perfect$ is reliable up to $\rankof{\anngvas}$.
    We first show that we can compute whether $\otherctxNGVAS{\anngvas}{\amarking_{\omega}, \anonterm, \amarkingp_{\omega}}$ has a pumping derivation.
    Since the choice of $i, j\in\concincount\cap\adimset$ was arbitrary, this implies that we can effectively check $(\amarking_{\omega}, \anonterm, \amarkingp_{\omega})\in\simplydecomps$. 
    Towards invoking \Cref{Lemma:EasilyComputableCG}, we argue that $\omegaof{\amarking_{\omega}}, \omegaof{\amarkingp_{\omega}}\supsetneq\omegaof{\acontextin}\cap\omegaof{\acontextout}$ holds.
    We know that $\omegaof{\acontextin}\subseteq\omegaof{\amarking_{\omega}}$.
    It is guaranteed that there is an $i\in\concincount\cap\adimset$ such that $i\in\omegaof{\amarking_{\omega}}, \omegaof{\amarkingp_{\omega}}$.
    Then, $\omegaof{\amarking_{\omega}}, \omegaof{\amarkingp_{\omega}}\supsetneq\omegaof{\acontextin}\supseteq\omegaof{\acontextin}\cap\omegaof{\acontextout}$.
    We invoke \Cref{Lemma:EasilyComputableCG} to construct $CG(\otherctxNGVAS{\anngvas}{\amarking_{\omega}, \anonterm, \amarkingp_{\omega}})$.
    Using this, we can check whether $\otherctxNGVAS{\anngvas}{\amarking_{\omega}, \anonterm, \amarkingp_{\omega}}$ admits a pumping derivation by \Cref{Lemma:WitnessGrammarTermination}.
    
    Let $(\amarking, \anonterm, \amarkingp)\in\simplydecomps$, and assume wlog. that $\otherctxNGVAS{\anngvas}{\amarking_{\omega}, \anonterm, \amarkingp_{\omega}}$ does not admit a pumping derivation.
    We show that $\postfuncNrof{\anngvas}{\concoutcount, \amarkingp}{\amarking, \anonterm}$ is decidable.
    As we argued, we can construct $CG(\otherctxNGVAS{\anngvas}{\amarking_{\omega}, \anonterm, \amarkingp_{\omega}})$.
    Since $\otherctxNGVAS{\anngvas}{\amarking_{\omega}, \anonterm, \amarkingp_{\omega}}$ also does not have pumping derivation, we can use \Cref{Proposition:WitnessGrammarDecomp} to get the decomposition $\adecomp$ of $\otherctxNGVAS{\anngvas}{\amarking_{\omega}, \anonterm, \amarkingp_{\omega}}$.
    As \Cref{Proposition:WitnessGrammarDecomp} yields a stronger decomposition, we even have $\rankof{\anngvasp}<\rankof{\anngvas}$ for all $\anngvasp\in\adecomp$.
    Our intention is to call $\perfect$ on the NGVAS in $\adecomp$ in order to get compute $\postfuncNr{\anngvas}{\concoutcount, \amarkingp}$.
    However, while moving from $\amarking$ to $\amarking_{\omega}$, we generalized our markings, this allowed more runs in $\runsof{\otherctxNGVAS{\anngvas}{\amarking_{\omega}, \anonterm, \amarkingp_{\omega}}}$ as we have in $\runsof{\otherctxNGVAS{\anngvas}{\amarking, \anonterm, \settoomega{\omegaoutcount}{\amarkingp}}}$.
    The latter system describes the runs we want to capture with $\postfuncNr{\anngvas}{\concoutcount, \amarkingp}$.
    To solve this issue, we reconcretize the markings.
    There is a small caveat, namely that the decomposition might have generated concrete markings that do not match $\amarking$ or $\settoomega{\omegaoutcount}{\amarkingp}$.
    In this case, we throw away these NGVAS, with the knowledge that they did not correspond to a fragment of $\runsof{\otherctxNGVAS{\anngvas}{\amarking, \anonterm, \settoomega{\omegaoutcount}{\amarkingp}}}$.
    We formalize these arguments.

    Let $\anngvasp\in\adecomp$, and let $\amarkingp^{\omegaoutcount}=\settoomega{\omegaoutcount}{\amarkingp}$ for brevity.
    If $\anngvasp.\acontextin\not\compwith\amarking$, or $\anngvasp.\acontextout\not\compwith\amarkingp^{\omegaoutcount}$, we argue $\runsof{\anngvasp}\cap\runsof{\otherctxNGVAS{\anngvas}{\amarking, \anonterm, \amarkingp^{\omegaoutcount}}}$.
    Suppose $\arun\in\runsof{\otherctxNGVAS{\anngvas}{\amarking, \anonterm, \amarkingp^{\omegaoutcount}}}\cap\runsof{\anngvasp}$.
    Let $\amarking\not\compwithat{i}\anngvasp.\acontextin$, the argument for $\amarkingp^{\omegaoutcount}\not\compwith\anngvasp.\acontextout$ is similar.
    We have $\anngvasp.\acontextin[i]\neq\amarking[i]$ and $\anngvasp.\acontextin[i], \amarking[i]\in\N$.
    Since $\anngvasp$ is a decomposition of $\otherctxNGVAS{\anngvas}{\amarking_{\omega}, \anonterm, \amarkingp_{\omega}}$, it must hold that $\amarking_{\omega}[i]=\omega$.
    Then 
    \begin{align*}
        \amarking[i]+\updates\cdot\paramparikhof{\updates}{\arun}&\sqsubseteq\amarkingp[i]\\
        \anngvasp.\acontextin[i]+\updates\cdot\paramparikhof{\updates}{\arun}&\sqsubseteq\anngvasp.\acontextout[i].
    \end{align*}
    Because $\anngvasp.\acontextin[i]\neq\amarking[i]$, then it must hold that $\amarkingp[i]=\omega$ or $\anngvasp.\acontextout[i]=\omega$.
    Assume $\amarkingp_{\omega}[i]\neq\omega$.
    Since $\anngvasp$ is a decomposition of $\otherctxNGVAS{\anngvas}{\amarking_{\omega}, \anonterm, \amarkingp_{\omega}}$, it must hold that $\anngvasp.\acontextout[i]\neq\omega$, which implies $\amarkingp[i]=\omega$.
    This contradicts the fact that $\amarkingp_{\omega}$ has more $\omega$'s.
    Conversely assume $\amarkingp_{\omega}[i]=\omega$.
    Then, $i\in\omegaof{\amarkingp_{\omega}}\cap\omegaof{\amarking_{\omega}}$.
    But in this case, the decomposition could not concretize $i$, which implies the contradiction $\anngvasp.\acontextin[i]=\omega$.
    
    Now let $\anngvasp\in\adecomp$ with $\anngvasp.\acontextin\compwith\amarking$ and $\anngvasp.\acontextout\compwith\amarkingp$.
    We define $\anngvasp_{\amarking, \amarkingp}$ to be the NGVAS with $\anngvasp_{\amarking, \amarkingp}.\acontextin$ the most concrete marking with $\anngvasp_{\amarking, \amarkingp}.\acontextin\sqsubseteq\amarking$, and $\anngvasp_{\amarking, \amarkingp}.\acontextin\sqsubseteq\anngvasp.\acontextin$, similarly for the output marking.
    We argue that $\runsof{\anngvasp_{\amarking, \amarkingp}}\subseteq\runsof{\otherctxNGVAS{\anngvas}{\amarking, \anonterm, \amarkingp^{\omegaoutcount}}}$.
    We already know that $\arun\in\runsof{\anngvasp_{\amarking, \amarkingp}}$ is enabled from $\amarking$.
    The language inclusions $\runsof{\anngvasp_{\amarking, \amarkingp}}\subseteq\runsof{\anngvasp}\subseteq\runsof{\otherctxNGVAS{\anngvas}{\amarking_{\omega}, \anonterm, \amarkingp_{\omega}}}\subseteq\runsof{\anonterm}$ deliver the desired result.
    Then, 
    $$\runsof{\otherctxNGVAS{\anngvas}{\amarking, \anonterm, \amarkingp^{\omegaoutcount}}}=\bigcup_{\anngvasp\in\adecomp,\;\anngvasp_{\amarking, \amarkingp}\text{ defined}}\runsof{\anngvasp_{\amarking, \amarkingp}}.$$ 
    Since we concretized the markings while moving from $\anngvasp$ to $\anngvasp_{\amarking, \amarkingp}$ and $\rankof{\anngvasp}<\rankof{\anngvas}$ already held for $\anngvasp\in\adecomp$, it also holds that $\rankof{\anngvasp_{\amarking, \amarkingp}}<\rankof{\anngvas}$ whenever $\anngvasp_{\amarking, \amarkingp}$ is defined.
    Then, we let 
    $$K=\setcond{\anngvasp'\in\unbdecomp_{\perfectnesssol}(\anngvasp_{\amarking, \amarkingp})}{\anngvasp\in\adecomp,\;\anngvasp_{\amarking, \amarkingp}\text{ defined}}$$
    to get an equivalent set of NGVAS where the invariant \perfectnesssol is established.
    Since $\adecomp$ was a decomposition and we did not modify the childNGVAS in $\anngvasp\in\adecomp$, \perfectnesschildren and \perfectnessbase are kept.
    By \Cref{Lemma:EstablishPerfSol}, the rank does not increase.
    Then, $\perfect$ is reliable for all $\anngvasp\in K$, and $\runsof{K}=\runsof{\otherctxNGVAS{\anngvas}{\amarking, \anonterm, \amarkingp^{\omegaoutcount}}}$.
    Therefore we can call $\perfect$ to compute the right hand side set
    $$\downclsof{\postfuncNrof{\anngvas}{\omegaoutcount, \amarkingp}{\amarking, \anonterm}}=\downclsof{\setcond{\anngvasp.\acontextout}{\anngvasp\in\perfectof{K}}}.$$
    This concludes the proof. 
\end{proof}

\begin{proof}[Proof of \Cref{Lemma:UWTCompleteness}]
    Consider a witness tree $\atree$ with $\omegaof{\atree.\inlabel}=\omegaof{\atree.\outlabel}$, $\atree.\inlabel=\amarkingin$, $\atree.\symlabel=\anonterminalin$.
    Since the witness trees are sound, and no pump has taken place, assume without the loss of generality that each leaf is a terminal.
    We can ensure this by appending the parse tree that witnesses $\amarking\fires{\anonterm}\amarkingp$ under a node labeled $(\amarking, \anonterm, \amarkingp)$.
    We work with the notion of workable witness trees.
    These are witness trees whose leaves are (depth 0) useful witness trees, or labeled with terminals.
    For a deepest node $\anode$ labeled $(\amarking, \asymbol, \amarkingp)$, with a non-useful witness tree below, we show that we can compute a useful witness tree $\atree_{use}$ with $\atree_{use}.\inlabel=\amarking$, $\atree_{use}.\symlabel=\asymbol$, and $\atree_{use}.\outlabel\geq\amarkingp$.
    This suffices to show our claim, since we can go from left-to-right and replace the non-useful subtree centered at each node $\anode$ with $\atree_{use}$, and propagate the difference $\atree_{use}-\amarkingp$ to the labels of the nodes that are placed to the right of $\atree_{use}$.
    
    Let $\asymbol=\aterm\in\terms$.
    Then, there must be $\amarkingp'\in\postfuncNof{\anngvas}{\amarking, \aterm}$ with $\amarkingp'\geq\amarkingp$.
    We let $\atree_{use}$ be the depth 0 useful witness tree labeled $(\amarking, \aterm, \amarkingp')$.
    Let $\asymbol=\anonterm\in\nonterms$, let $\amarking\not\in\domain$, and $(\amarking, \anonterm, \amarkingp)\in\simplydecomps$.
    Then, similarly to the previous case, $\amarkingp'\in\postfuncNrof{\anngvas}{\concoutcount, \amarkingp}{\amarking, \aterm}$ with $\amarkingp'\geq\amarkingp$ exists.
    We let $\atree_{use}$ once more be the depth 0 useful witness tree labeled $(\amarking, \aterm, \amarkingp')$.
    Now, let $\asymbol=\anonterm\in\nonterms$, let $\amarking\not\in\domain$, but $(\amarking, \anonterm, \amarkingp)\not\in\simplydecomps$.
    Since $\atree$ is a witness tree with $\atree.\inlabel=\amarkingin$, and $\atree.\symlabel=\anonterminalin$, we know that $\booleanflagof{\domain}=\top$ must hold.
    Then, get an equation-maximal $(\amarking, \anonterm, \amarkingp')$ with $\amarkingp'\geq\amarkingp$.
    This must exist since $(\amarking, \anonterm, \amarkingp)$ is soundly labeled.
    The construction of $\atree_{use}$ is the same.
    The case where $\asymbol=\anonterm\in\nonterms$ and $\omegaincount\subsetneq\omegaof{\amarking}$ is also similar, but we call $\postfuncNof{\anngvas}{\amarking, \anonterm}$ instead of $\postfuncNrof{\anngvas}{\omegaoutcount}{\amarking, \anonterm}$.

    Now let $\asymbol=\anonterm\in\nonterms$, but conversely let $\amarking\in\domain$.
    Then, for the subtree $\atreep$ centered on $\anode$, $\amarkingp\neq\pumpingof{\atreep}.\outlabel$ must hold, or $\atreep$ has a successor with the same labeling.
    In the former case, we have $\amarkingp<\pumpingof{\atreep}.\outlabel$ by the definition of $\pumpingof{\atreep}$.
    Since $\anode$ is a deepest node, where the subtree below is not a useful witness tree, all strict subtrees must be useful witness trees.
    Then, we let $\atree_{use}$ be $\pumpingof{\atreep}$.
    We have $\pumpingof{\atreep}.\inlabel=\atreep.\inlabel=\amarking$ and $\pumpingof{\atreep}.\symlabel=\atreep.\symlabel=\anonterm$.
    In the latter case, we just let $\atree_{use}=\atreep'$ for the subtree of $\atreep$ that has the same root labeling.
    We know that $\atree_{use}=\atreep'$ has the same root labeling as $\atreep$.
    Also, by a similar argument to the former case, we know that $\atree_{use}$ is a useful witness tree.
    This concludes the proof.
\end{proof}

\begin{proof}[Proof of \Cref{Lemma:UWTVerification}]
    We construct the witness trees in $\witnessset^{(i)}$ inductively in $i\in\N$.
    We have $\witnessset^{(0)}=\emptyset$ for the base case, since there are no useful witness trees that have a leaf labeled $(\amarking, \anonterm, \amarkingp)$, with $\amarking\in\domain$.
    In order to construct $\witnessset^{(i+1)}$ we use the trees we gathered in $\witnessset^{(i)}$, the computability of $\postfuncNr{\anngvas}{\concoutcount, \amarkingp}$, and \Cref{Lemma:UsefulRestriction}.
    We define the function $\knownoutputs{i}:\Nomega^{(i+1)}\times\terms\cup\nonterms\to\powof{\usefultrees}$ which delivers the set of useful witness trees with depth at most $i$, and the input value and the symbol as inputted into $\knownoutputs{i}$.
    We argue that the function $\knownoutputs{i}$ is computable, given that the premise of the lemma holds, and $\witnessset^{(i)}$ is provided.
    We use $\knownoutputs{i}$ to construct $\witnessset^{(i+1)}$.

    We proceed by the computability argument of $\knownoutputs{i}$.
    We let 
    $$\knownoutputsof{i}{\amarking, \aterm}=\setcond{(\amarking, \aterm, \amarkingp)}{\amarkingp\in\postfuncNof{\anngvas}{\amarking, \aterm}}$$
    for all $\aterm\in\terms$ and $i\in\N$.
    We use the labeling triple e.g. $(\amarking, \aterm, \amarkingp)$ to denote the depth 0 tree with said label. 
    For $\amarking\in\Nomega$ with $\amarking\not\in\domain$ and $\omegaof{\amarking}=\omegaincount$, we let $\knownoutputsof{i}{\amarking, \anonterm}$ be 
    \begin{align*}
        \setcond{(\amarking, \anonterm, \amarkingp')&}{\amarkingp'\in \;\postfuncNrof{\anngvas}{\concoutcount, \amarkingp}{\amarking, \anonterm}\\
        &(\amarking, \anonterm, \amarkingp)\in\simplydecomps\text{ equation justified},\;\omegaof{\amarkingp}=\omegaoutcount}
    \end{align*}
    if $\booleanflagof{\domain}=\bot$.
    We do not restrict ourselves with $\omegaof{\amarkingp}=\omegaoutcount$, since these are the only relevant counters for $\postfuncNr{\anngvas}{\concoutcount, \amarkingp}$.
    Furthermore, because $(\amarking, \anonterm, \amarkingp)$ is equation-justified, and $\concoutcount$ precisely the output counters that are not in the support of the homogeneous equation, there are only finitely many $\amarkingp$ values, and we can compute them.
    Since $\postfuncNr{\anngvas}{\omegaoutcount, \amarkingp}$ is computable by \Cref{Lemma:SimplyDecomposable} under our assumptions, and the set of fitting $\amarkingp$ is finite and computable, $\knownoutputsof{i}{\amarking, \anonterm}$ is computable.
    If $\booleanflagof{\domain}=\top$ holds, we let 
    $$\knownoutputsof{i}{\amarking, \anonterm}=\setcond{(\amarking, \anonterm, \amarkingp)}{(\amarking,\anonterm, \amarkingp)\text{ equation-maximal}}$$
    for the same $\amarking$ and $\anonterm$.
    Next, if $\amarking\not\in\domain$ but $\omegaincount\subsetneq\omegaof{\amarking}$, we let
    $$\knownoutputsof{i}{\amarking, \anonterm}=\setcond{(\amarking, \anonterm, \amarkingp)}{\amarkingp\in\postfuncNof{\anngvas}{\amarking, \anonterm}}.$$
    The function $\postfuncNof{\anngvas}{\amarking, \anonterm}$ is computable for $\omegaincount\subsetneq\omegaof{\amarking}$, because for the NGVAS $\anngvasp_{\postfuncNof{\anngvas}{\amarking, \anonterm}}$ that corresponds to this query, the first component of $\rankof{\anngvasp_{\postfuncNof{\anngvas}{\amarking, \anonterm}}}$ is at most $d-\cardof{\omegaincount}-1$, while the first component of $\rankof{\anngvas}$ is, $d-\cardof{\omegaof{\acontextin}\cap\omegaof{\acontextout}}$ which is at least $d-\cardof{\omegaincount}$.
    Finally, let $\amarking\in\domain$, and $\anonterm\in\nonterms$.
    In this case, we let 
    $$\knownoutputsof{i}{\amarking, \anonterm}=\setcond{\atree\in\witnessset^{(i)}}{\atree.\inlabel=\amarking,\;\atree.\symlabel=\anonterm}.$$
    
    With $\knownoutputsof{i}{\amarking, \anonterm}$ at hand, the construction of $\witnessset^{(i+1)}$ is straightforward.
    First, we include $\witnessset^{(i)}$ in $\witnessset^{(i+1)}$.
    Then, we iterate over all $\amarking\in\domain$, $\anonterm\in\nonterms$, rule $\anonterm\to\asymbol.\asymbolp$ in $\prods$, $\atree_{left}\in\knownoutputsof{i}{\amarking, \asymbol}$, and $\atree_{right}\in\knownoutputsof{i}{\atree_{left}.\outlabel, \asymbolp}$.
    At each iteration, we construct the witness tree $\atreep=\pumpingof{\atree}$, where $\atree$ has $\atree_{left}$ as its left child, $\atree_{right}$ as its right child, $\atree.\inlabel=\atree_{left}.\inlabel$, and $\atree.\outlabel=\atree_{right}.\outlabel$.
    Since all its subtrees are useful witness trees and $\atreep.\inlabel\in\domain$, $\atreep$ is a useful witness tree if and only if no two successors share the same labeling.
    We check this, and let $\atreep\in\witnessset^{(i+1)}$ if $\atreep$ is indeed a useful witness tree.
    Clearly, this construction captures all useful witness trees $\atree$ with depth at most $i+1$, $\atree.\inlabel\in\domain$, and $\atree.\symlabel\in\nonterminals$. 
\end{proof}

\begin{proof}[Proof sketch for \Cref{Lemma:UWTFPStabilization}]
    Let $\witnessset^{(i)}=\witnessset^{(i+1)}$, and let $\atree\in\witnessset^{(i+2)}$.
    If the subtree rooted at a child is a useful witness tree with input label in $\domain$, then it is has depth at most $i+1$, and therefore is in $\witnessset^{(i+1)}=\witnessset^{(i)}$.
    If the the input label of a subtree rooted at a child is not in $\domain$, then it is a depth 0 subtree.
    Therefore, $\atree$ has depth $i+1$, meaning which implies $\atree\in\witnessset^{(i+1)}$. 
\end{proof}

\begin{proof}[Proof of \Cref{Lemma:UWTFPGuaranteedStabilization}]
    Suppose that $\witnessset^{(i)}\neq\witnessset^{(i+1)}$ for all $i\in\N$.
    This implies that for each $i\in\N$, there is a $\atree\in\witnessset^{(i+1)}\setminus\witnessset^{(i)}$.
    Let $\usefultrees=\bigcup_{i\in\N}\witnessset^{(i)}$.
    Consider the graph $H=(Y, E)$, where $H\subseteq\N\times\usefultrees$ with $(i, \atree)\in Y$ if and only if $\atree\in\witnessset^{(i)}\setminus\witnessset^{(i-1)}$, and $((i, \atree), (i', \atree'))\in E$, if and only if $i'=i+1$, and $\atree$ is a subtree of $\atree'$.
    It must hold that $H$ is infinite.
    Clearly, any $(i+1, \atree)\in Y$ with $i\geq 1$ has a predecessor $(i, \atreep)\in Y$.
    If this did not hold, then the contradiction $\atree\in\witnessset^{(i)}$ would hold.
    Since $\witnessset^{(1)}$ is finite, there are only finitely many $(1, \atree)\in Y$.
    This means that all nodes are connected to at least one node in a finite set of nodes.
    So, $H$ only has finitely many components.
    Since $\witnessset^{(i)}$ is finite for all $i\in\N$, and any edge connects nodes between adjacent levels, $(H, E)$ is finitely branching.
    We apply Koenig's Lemma to get a sequence $[(i, \atree_{i})]_{i\in\N_{\geq N}}$ in $H$ with $((i, \atree_{i}), (i+1, \atree_{i+1}))\in E$ for all $i\in\N_{\geq N}$.
    This implies that for all $i\in\N_{\geq N}$, $\atree_{i}$ has depth $i$, and that it is a subtree of $\atree_{i+1}$.
    Using the fact that $\Nomega^{d}$ is a WQO and that $\domain$ is finite, we get a subsequence $[(\phi(i), \atreep_{i})]_{i\in\N}$ of $[(i,\atree_{i})]_{i\in\N_{\geq N}}$, where $\atreep_{i}.\inlabel$ and $\atreep_{i}.\symlabel$ are constant across $i\in\N$, and $\atreep_{i}.\outlabel\leq\atreep_{i+1}.\outlabel$ for all $i\in\N$.
    Also, since $\atreep_{i}$ is a subtree of $\atreep_{i+1}$, and no node may have the same labeling as its successor, we know that $\atreep_{i}.\outlabel<\atreep_{i}.\outlabel$ must hold for all $i\in\N$.
    But since $\atreep_{i}.\inlabel=\atreep_{i+1}.\inlabel$, and $\atreep_{i}.\symlabel=\atreep_{i+1}.\symlabel$, we must have some $j\leq d$ with $\atreep_{i}.\outlabel[j]<\atreep_{i+1}.\outlabel[j]$, which implies $\pumpingof{\atreep_{i+1}}.\outlabel[j]=\omega$.
    As a consequence, we get $|\omegaof{\atreep_{i}}|<|\omegaof{\atreep_{i+1}}|$.
    Then, $[|\omegaof{\atreep_{i}}|]_{i\in\N}$ must grow unboundedly.
    This is a contradiction to $|\omegaof{\atreep_{i}}|\leq d$.
\end{proof}

%-------------------------------------------------------------------------------------------------------------------
%-------------------------------------------------------------------------------------------------------------------
%-------------------------------------------------------------------------------------------------------------------

\subsection{Proving \Cref{Lemma:UsefulRestriction} (Computing $\domainconst$)}\label{Section:ComputingDPlus}
We show that we can compute a $\domainconst\in\N$ with the properties stated in the lemma.
The reliability assumptions on $\perfect$ and assumptions on properties of $\anngvas$ carry over.
In order to effectively construct $\domainconst$, we need to compute a few key values for $\anngvas$.
In the following, we use $\otherctxNGVAS{\anngvas}{\amarking, \anonterm, \amarkingp}$ having a pumping derivation and $(\amarking, \anonterm, \amarkingp)$ having a pumping derivation exchangeably.
We refer to $(\amarking, \anonterm, \amarkingp)\in\nonterms$ as a \emph{marking}, if $\amarking\sqsubseteq\inof{\anonterm}$ and $\amarkingp\sqsubseteq\outof{\anonterm}$.
We write $\cteffectof{\arunp}\in\Z^{d}$ to denote $\sum_{\anupd\in\updates}\at{\paramparikhof{\updates}{\arun}}{\anupd}\cdot\anupd$.
For $\arun\in\updates^{*}$ we write $\sizeof{\arun}=\sum_{i\leq \cardof{\arun}}\sizeof{\arun[i]}$, where $\sizeof{\avec}$ is the $1$-norm for the vector $\avec\in\Z^{*}$.
We postpone the proof of \Cref{Proposition:Precalculation} until we have proven \Cref{Lemma:UsefulRestriction}.

\begin{proposition}\label{Proposition:Precalculation}
    We can compute
    \begin{itemize}
        \item a set $\extcovmap\subseteq\N^{d}\times\nonterms\times\N^{d}$ where a marking $(\amarking, \anonterm, \amarkingp)$ with $\amarking[i]=\amarkingp[j]=\omega$ for some $i, j \in\concincount$, and $\omegaincount\subseteq\omegaof{\amarking}$, $\omegaoutcount\subseteq\omegaof{\amarkingp}$, has a pumping derivation if and only if $(\amarking,\anonterm, \amarkingp)\in\upclsof{\extcovmap}$.
        \item a number $\extcovconst\in\N$ where for all $(\amarking, \anonterm, \amarkingp)\in\extcovmap$, there is a pumping derivation of $\sizeof{.}$-size at most $\extcovconst$
        \item  a number $\incconst\in\Nomega$ where for all $\anonterm\in\nonterms$, if $\incconst\neq\omega$, there is a derivation $\anonterm\to\asentform.\anonterm.\asentformp$ with $\arun\in\runsof{\asentform}$, $\arunp\in\runsof{\asentformp}$, and $\at{\cteffectof{\arun}}{i}\geq 1$, $-\at{\cteffectof{\arunp}}{j}\geq 1$  for all $i\in\adimset\setminus\omegaoutcount$  and $j\in\adimset\setminus\omegaincount$, where $\sizeof{\arun}, \sizeof{\arunp}\leq\incconst$. 
        If $\incconst\neq\omega$, there is no such derivation.
        \item a number $\excconst\in\Nomega$ where for all $\anonterm,\anontermp\in\nonterms$, there is a derivation $\anonterm\to\asentform.\anontermp.\asentformp$ with $\arun\in\runsof{\asentform}$, $\arunp\in\runsof{\asentformp}$ and $\cardof{\arun},\cardof{\arunp}\leq\excconst$.
    \end{itemize} 
\end{proposition}

We further define a set $\agreefuncof{\extcovmap}$ which overapproximates all markings that may admit an external covering sequence.
\begin{align*}
    \agreefuncof{\extcovmap}=&\upclsof{\extcovmap}\cup\setcond{(\amarking,\anonterm,\amarkingp)}{\text{for all }i, j\in\concincount,\\
    &\hspace{4.0em} (\settoomega{\amarking}{i\cup\omegaincount}, \anonterm, \settoomega{\amarkingp}{j\cup\omegaoutcount})\in\upclsof{\extcovmap}}
\end{align*}
This set is the complement of the set of simply decomposable nodes, since by definition $(\amarking, \anonterm, \amarkingp)\not\in\agreefuncof{\extcovmap}$ indicates that a lower dimensional $\extcovnl$ call will yield a decomposition.

\begin{lemma}\label{Lemma:EasyDecomposition}
    Let $(\amarking, \anonterm, \amarkingp)$ be a marking with $\omegaincount\subseteq\omegaof{\amarking}$ and $\omegaoutcount\subseteq\omegaof{\amarkingp}$.
    We have $(\amarking, \anonterm, \amarkingp)\in\simplydecomps$ if and only if $(\amarking, \anonterm, \amarkingp)\not\in\agreefuncof{\extcovmap}$.
\end{lemma}

The lemma \Cref{Lemma:UsefulRestriction} states two cases, depending on $\booleanflagof{\domain}$.
We let $\booleanflagof{\domain}=\top$ if and only if $\incconst\in\N$. 
We make a case distinction on $\booleanflagof{\domain}$.\\

\noindent\textit{Case $\booleanflagof{\domain}=\top$.} Our goal is to find a pumping derivation for equation maximal $(\amarking, \anonterm, \amarkingp)\not\in\simplydecomps$, $\omegaof{\amarking}=\omegaincount$, where one counter of $\amarking$ is very large.
Since equation maximality allows $\omega$'s for the output counters that are in the support of the homogeneous equation of $\otherctxNGVAS{\anngvas}{\amarkingin, \anonterminalin, \outof{\anonterm}}$, and the homogeneous systems of $\otherctxNGVAS{\anngvas}{\amarking, \anonterm, \outof{\anonterm}}$ and $\otherctxNGVAS{\anngvas}{\amarkingin, \anonterminalin, \outof{\anonterm}}$ are the same, we get $\amarkingp=\omegaoutcount$.
We will argue that the perfectness assumptions for $\anngvas$ carries over to $\otherctxNGVAS{\anngvas}{\amarking, \anonterm, \amarkingp}$, which yields $\amarking\fires{\runsof{\anonterm}}\amarkingp$ when combined with the pumping derivation and \Cref{TheoremGVASReachDecidable}. 
We observe that the perfectness conditions carry over.

\begin{lemma}\label{Lemma:PerfectnessCarryOver}
    Let $\anngvas$ have all the perfectness conditions but \perfectnesspumpingnospace, and $(\amarking, \anonterm, \amarkingp)$ a marking with $\omegaof{\amarking}=\omegaincount$ and $\omegaof{\amarkingp}=\omegaoutcount$.
    Then, $\otherctxNGVAS{\anngvas}{\amarking, \anonterm, \amarkingp}$ also has all the perfectness conditions but \perfectnesspumpingnospace.
\end{lemma}

\begin{proof}
    Let $(\amarking, \anonterm, \amarkingp)$ as described in the lemma.
    We argue condition by condition that perfectness holds for $\otherctxNGVAS{\anngvas}{\amarking, \anonterm, \amarkingp}$.
    The condition \perfectnesssol holds by definition.
    Since childNGVAS of $\otherctxNGVAS{\anngvas}{\amarking, \anonterm, \amarkingp}$ and $\anngvas$ are the same, \perfectnesschildren and \perfectnessbase are both fulfilled.
    We know that $\omegaoutcount$ is precisely the set of output counters in the support of $\otherctxNGVAS{\anngvas}{\amarkingin, \anonterminalin, \outof{\anonterminalin}}$.
    Because $\omegaof{\amarkingin}=\omegaincount$, the homogeneous systems of $\otherctxNGVAS{\anngvas}{\amarking, \anonterm, \outof{\anonterm}}$ and $\otherctxNGVAS{\anngvas}{\amarking, \anonterm, \outof{\anonterm}}$.
    Then, $\omegaoutcount=\omegaof{\amarkingp}$ is precisely the set of counters in the support of $\otherctxNGVAS{\anngvas}{\amarking, \anonterm, \outof{\anonterm}}$.
    This means that $\otherctxNGVAS{\anngvas}{\amarking, \anonterm, \amarkingp}$ fulfills \perfectnesscountersnospace.
    Finally we consider \perfectnessprods and \perfectnesschildperiodsnospace.
    Since these conditions hold for $\anngvas$, we know that there is a homogeneous solution $\asol$ to $\homchareq{\anngvas}$ where $\at{\asol}{i}=0$ for all $i\not\in\omegaof{\acontextin}\supseteq\omegaincount$, and $\at{\asol}{\aprod}\geq 1$ and $\at{\asol}{\aperiod}\geq 1$ for all $\aprod\in\prods$ and child periods $\aperiod$.
    Then, $\asol$ also solves the homogeneous equation of $\otherctxNGVAS{\anngvas}{\amarking, \anonterm, \outof{\anonterm}}$.
    This implies that $\at{\asol}{i}=0$ for all $i\in\concoutcount$.
    Then, $\asol$ solves the homogeneous equation of $\otherctxNGVAS{\anngvas}{\amarking, \anonterm, \amarkingp}$ as well.

\end{proof}

Thanks to \Cref{Lemma:PerfectnessCarryOver}, if we find a pumping derivation, then \Cref{TheoremIterationLemmaNonLinearOverview} applies and shows $\amarking\fires{\runsof{\anonterm}}\amarkingp$.
The set $\extcovmap$ brings us very close to this goal: Only one counter remains unaccounted for in the pumping derivations implied by this set.
To fully achieve our goal, we combine the derivation implied by $\incconst\in\N$ with the derivation implied by $\extcovmap$.
We apply the sequence implied by $\extcovmap$ until the counters considered by $\extcovmap$ are large enough to enable the $\incconst$ derivation.
From this point, we can iterate $\incconst$ unboundedly. 
In order to do this, we need one counter on either side of the marking to be large enough the withstand the initial $\extcovmap$ derivations.
In the rest of the section, we write $\fires{\arun}_{(i)}$ to denote that the run $\arun$ is enabled for counter $i$.

\begin{lemma}\label{Lemma:GuaranteedPump}
    Let $\booleanflagof{\domain}=\top$.
    Further let $(\amarking, \anonterm, \amarkingp)$ be a marking with $(\amarking, \anonterm, \amarkingp)\not\in\simplydecomps$, $\omegaof{\amarking}=\omegaincount$, $\omegaof{\amarkingp}=\omegaoutcount$, and $\amarking[i], \amarkingp[j]\geq\posconst$ for $i, j\in\concincount$ where $\posconst=\incconst\cdot\extcovconst+\incconst$.
    Then, $\amarking\fires{\runsof{\anonterm}}\amarkingp$.
\end{lemma}

\begin{proof}
    Let $(\amarking, \anonterm, \amarkingp)$, $\posconst$, and $\booleanflagof{\domain}$ be as given in the lemma.
    We show that $(\amarking, \anonterm, \amarkingp)$ admits a pumping derivation.
    Then, by \Cref{Lemma:PerfectnessCarryOver}, we can apply \Cref{TheoremIterationLemmaNonLinearOverview} and get $\amarking\fires{\runsof{\anonterm}}\amarkingp$.
    We argue that there is a derivation $\anonterm\to\asentform.\anonterm.\asentformp$ with $\arun\in\runsof{\asentform}$, $\arunp\in\runsof{\asentformp}$, $\amarking\fires{\arun}\amarking'$, $\amarkingp'\fires{\arunp}\amarkingp$, with $\amarking'\geq \incconst \cdot 1_{\concincount}$ and $\amarkingp'\geq \incconst \cdot 1_{\concoutcount}$.
    This is because from this point the $\incconst$-derivation $\anonterm\to\asentform_{\incconst}.\anonterm.\asentformp_{\incconst}\to\arun_{\incconst}.\anonterm.\arunp_{\incconst}$ implied by $\incconst\in\N$ can be taken until all relevant counters are increased arbitrarily.
    In the following, we assume $j\in\concoutcount$ to prove the more involved case.
    If $j\not\in\concoutcount$, the same proof applies with the arguments for the output side removed, since we would have $\at{\amarkingp}{j}=\omega$ and thus nothing to show for the derivation on this side.
    First, note that $(\amarking, \anonterm, \amarkingp)\in\agreefuncof{\extcovmap}$, implies that $(\settoomega{i\cup\omegaincount}{\amarking}, \anonterm, \settoomega{j\cup\omegaoutcount}{\amarkingp})$ admits a pumping sequence, that is, 
    $$\anonterm\to\asentform_{\mathsf{pump}}.\anonterm.\asentformp_{\mathsf{pump}},$$
    where $\arun_{\mathsf{pump}}\in\runsof{\asentform_{\mathsf{pump}}}$, $\arunp_{\mathsf{pump}}\in\runsof{\asentformp_{\mathsf{pump}}}$ with $\amarking[i']\fires{\arun_{\mathsf{pump}}}_{(i')}\amarking[i']+b$, $\amarkingp[j']+c\fires{\arunp_{\mathsf{pump}}}_{(j')}\amarkingp[j']$, and $b, c\geq 1$ for all $i'\in\omegaincount\setminus\set{i}$ and $j'\in\omegaoutcount\setminus\set{j}$.
    We can further assume $\sizeof{\arun_{\mathsf{pump}}}, \sizeof{\arun_{\mathsf{pump}}}\leq\extcovconst$ by the definition of $\extcovconst$.
    Then, consider the derivation 
    $$\anonterm\to\asentform_{\mathsf{pump}}.\anonterm.\asentformp_{\mathsf{pump}}\to\arun_{\mathsf{pump}}^{\incconst}.\anonterm.\arunp_{\mathsf{pump}}^{\incconst}$$
    We already have 
    $$\amarking[i']\fires{\arun_{\mathsf{pump}}}_{(i')}\amarking[i']+\incconst\cdot b,\;\;  \amarking[i']+\incconst\cdot b\geq \incconst\cdot b\geq \incconst$$ 
    for all $i'\in\omegaincount\setminus\set{i}$.
    Similarly, $\amarkingp[j']+ c\cdot\incconst\fires{\arunp_{\mathsf{pump}}}_{(j')}\amarkingp[j']$ and $\incconst\leq \amarkingp[j']+ c\cdot\incconst$ for all $j'\in\omegaoutcount\setminus\set{j}$.
    Since $\cardof{\asentform_{\mathsf{pump}}}, \cardof{\asentformp_{\mathsf{pump}}}\leq \extcovconst$, we have 
    \begin{align*}
        R=\incconst\cdot\extcovconst+\incconst\geq\incconst\cdot\extcovconst\geq \incconst\cdot\cardof{\asentform_{\mathsf{pump}}}, \incconst\cdot\cardof{\asentformp_{\mathsf{pump}}} 
    \end{align*}
    which means that effects on counter $i$ are enabled forwards from $\amarking[i]$, and effects on counter $j$ are enabled backwards from $\amarkingp[j]$.
    We observe
    \begin{align*}
        R-\incconst\cdot\cardof{\asentform_{\mathsf{pump}}}\geq\incconst \qquad R-\incconst\cdot\cardof{\asentformp_{\mathsf{pump}}}\geq\incconst
    \end{align*}
    which means that $\amarking[i]\fires{\arun_{\mathsf{pump}}}_{(i)} h$ and $g\fires{\arunp_{\mathsf{pump}}}_{(j)}\amarkingp[j]$ for $h, g\geq \incconst$.
\end{proof}

We now show that if $(\amarking, \anonterm, \amarkingp)$ is equation-maximal, then we only need the input counter to be large.
We write $\solthresholdof{k}$ to be the size of the largest basis solution of an integer linear system of size at most $k\in\N$, which can be computed in elementary time.
\Cref{Lemma:OneSideGuaranteesPump} implies \Cref{Lemma:UsefulRestriction} in the $\booleanflagof{\domain}=\top$ case.

\begin{lemma}\label{Lemma:OneSideGuaranteesPump}
    Let $(\amarking, \anonterm, \amarkingp)\not\in\simplydecomps$ be an equation-maximal marking with $\omegaof{\amarking}=\omegaincount$, and let $\booleanflagof{\domain}=\top$.
    If $\amarking[i]\geq \solthresholdof{\bigoof{d\cdot\posconst}+\cardof{\chareq{\anngvas}}}+1$ for $\posconst$ as defined in \Cref{Lemma:GuaranteedPump} and some $i\in\concincount$, then $\amarking\fires{\runsof{\anonterm}}\amarkingp$.
\end{lemma}

\begin{proof}
    Let $(\amarking, \anonterm, \amarkingp)$ and $\posconst$ be as defined in the lemma.
    We have $\omegaof{\amarkingp}=\omegaoutcount$ by the definition of equation-maximality.
    If $\concoutcount\neq\concincount$ and therefore $\concoutcount\subset\concincount$, we can pick $j\in\concoutcount$ and get $\amarkingp[j]=\omega\geq R$.
    Then let $\concoutcount=\concincount$.
    Suppose that for all $j\in\concoutcount$, $\amarkingp[j]<\posconst$ holds.
    We show that in this case, $(\amarking, \anonterm, \amarkingp)$ is not equation-maximal.
    Consider the characteristic equation of $\otherctxNGVAS{\anngvas}{\inof{\anonterm}, \anonterm, \amarkingp}$.
    The size of this characteristic equation is at most $\bigoof{d\cdot\posconst}+\cardof{\chareq{\anngvas}}$ the size of the characteristic equation $\cardof{\chareq{\anngvas}}$ for $\anngvas$, and $\bigoof{d}$ additional constraints.
    Then, since $(\amarking, \amarkingp)$ forms a part of the solution to the characteristic equation of $\otherctxNGVAS{\anngvas}{\inof{\anonterm}, \anonterm, \amarkingp}$, we have $\amarking=b+c_{\mathsf{hom}}$ for some $b,c_{\mathsf{hom}}\in\N^{d}$ where $b$ solves the equation as well, and $b[i]\leq \solthresholdof{\bigoof{d\cdot\posconst}+\cardof{\chareq{\anngvas}}}$ for all $i\leq d$.
    Because $\amarking[i]\geq \solthresholdof{\bigoof{d\cdot\posconst}+\cardof{\chareq\anngvas}}+1$ for some $i\in\concincount$, we have $c_{\mathsf{hom}}[i]\geq\posconst$.
    We know that $(b, \amarkingp)$ can be specialized into the input and output markings for a solution to the marking equation for $\otherctxNGVAS{\anngvas}{\inof{\anonterm}, \anonterm, \outof{\anonterm}}$.
    Then, so must $(b+c_{\mathsf{hom}}, \amarkingp+c_{\mathsf{hom}})=(\amarking, \amarkingp+ c_{\mathsf{hom}})$ have this property.
    Since $c_{\mathsf{hom}}\neq 0$, this implies that $(\amarking, \anonterm, \amarkingp)$ was not equation-maximal.
\end{proof}

\noindent\textit{Case $\booleanflagof{\domain}=\bot$.}
We move on to the second case of the lemma.
The strategy is to deduce a derivation that would imply $\incconst\neq\omega$ if a counter in the input marking of a witness tree with root label $(\amarkingin, \anonterminalin, \amarkingp)$ grows too large.
We make a distinction between the cases $\concoutcount\subset\concincount$ and $\concoutcount=\concincount$.
For the case $\concoutcount\subseteq\concincount$, we just follow the proof strategy we laid out.
For the $\concoutcount=\concincount$, we show the same result, but we additionally need to assume that $\nodemarkingof{\anode}$ has an output value that grows too large.
Then, we show that in the $\concoutcount=\concincount$ case, the output values cannot diverge too far below input values, showing our result.

\begin{lemma}\label{Lemma:GuaranteedContradictionSimple}
    Let $\booleanflagof{\domain}=\bot$.
    Let $\atree$ be a witness tree with root label $(\amarkingin, \anonterminalin, \amarkingp)$ and $\omegaof{\amarkingin}=\omegaincount$, let $\concoutcount\subset\concincount$, and let $\abigconst=\sum_{j\in\concincount}\cardof{\amarkingin[j]}+\sum_{j\in\concoutcount}\cardof{\amarkingp[j]}$.
    Further let $\atree$ contain a node labeled $(\amarking, \anonterm, \amarkingpp)$, where $\amarking[i]\geq\negconst$ for $\negconst=(\extcovconst+\abigconst+1)\cdot(\extcovconst+1)$, , and $i\in\concincount$.
    Then, $(\amarking, \anonterm, \amarkingpp)\in\simplydecomps$.
\end{lemma}

\begin{proof}
    Suppose there is a witness tree $\atree$ with root labeled $(\amarkingin, \anonterminalin, \amarkingp)$, and let there be a node $\anode$ in $\atree$ labeled $(\amarking, \anonterm, \amarkingpp)$ with $(\amarking, \anonterm, \amarkingpp)\not\in\simplydecomps$, but $\amarking[i]\geq\negconst$ for some $i\in\concincount$.
    First, the soundness of witness trees imply a derivation 
    $$\anonterminalin\to \asentform_{0}.\anonterm.\asentformp_{0}\to\arun_{0}.\anonterm.\arunp_{0}$$
    where $\asentform_{0}, \asentformp_{0}\in\terms^{*}$, $\arun_{0}\in\runsof{\asentform_{0}}$, $\arunp_{0}\in\runsof{\asentformp_{0}}$, $\amarkingin[i]+\cteffectof{\arun_{0}}[i]\geq \negconst$, and $\amarking[i']+\cteffectof{\arun_{0}}[i']\geq 0$ for all $i'\in\concincount$.
    Because of $\omegaof{\amarkingpp}\subseteq\omegaoutcount$, we can also assume $\amarkingp[j']+\cteffectof{\arunp_{0}}[j']\geq 0$.
    This gives us $\cteffectof{\arun_{0}}[i']\geq -\abigconst+1$, and $\cteffectof{\arunp_{0}}[j']\geq \abigconst-1$ by the defintion of $\abigconst$ for all $i'\in\concincount\setminus\set{i}$, $j'\in\concoutcount\setminus\set{j}$.
    We also get $\cteffectof{\arun_{0}}[i]\geq \negconst-\abigconst+1$.
    Since $\concoutcount\subset\concincount$, choose $j\in\concincount\setminus\concoutcount$.
    Because $(\amarking, \anonterm, \amarkingpp)\not\in\simplydecomps$, we know that there is a derivation 
    $$\anonterminalin\to\asentform_{1}.\anonterm.\asentformp_{1}\to\arun_{1}.\anonterm.\arunp_{1}$$
    that pumps certain counters, where $\asentform_{1}, \asentformp_{1}\in\terms^{*}$, $\arun_{1}\in\runsof{\asentform_{1}}$, $\arunp_{1}\in\runsof{\asentformp_{1}}$.
    Then, $\cteffectof{\arun_{1}}[i']\geq 1$, $\cteffectof{\arunp_{1}}[j']\geq 1$ for all $i'\in\concincount\setminus\set{i}$ and $j'\in\concincount\setminus\set{j}\supseteq\concoutcount$.
    We combine these two derivations with the following derivation implied by $\excconst$:
    $$\anonterm\to\asentform_{\excconst}.\anonterminalin.\asentformp_{\excconst}\to\arun_{\excconst}.\anonterm.\arunp_{\excconst}$$
    where $\asentform_{\excconst}, \asentformp_{\excconst}\in\terms^{*}$, $\arun_{\excconst}\in\runsof{\asentform_{\excconst}}$, $\arunp_{\excconst}\in\runsof{\asentformp_{\excconst}}$.
    We also have $\cardof{\arun_{\excconst}}, \cardof{\arunp_{\excconst}}\leq\excconst$.
    This allows us to get back to $\anonterminalin$.
    In total, we get
    \begin{align*}
        \anonterminalin
        &\to\asentform_{0}.\asentform_{1}^{\abigconst+\excconst}.\anonterm.\asentformp_{1}^{\abigconst+\excconst}.\asentformp_{1}\\
        &\to\asentform_{0}.\asentform_{1}^{\abigconst+\excconst}.\asentform_{\excconst}.\anonterminalin.\asentformp_{\excconst}.\asentformp_{1}^{\abigconst+\excconst}.\asentformp_{1}\\
        &\to\arun_{0}.\arun_{1}^{\abigconst+\excconst}.\arun_{\excconst}.\anonterminalin.\arunp_{\excconst}.\arunp_{1}^{\abigconst+\excconst}.\arunp_{0}
    \end{align*}
    The total effect on counter $i$ from the left is at least $\negconst-\abigconst+1-(\abigconst+\excconst)\cardof{\arun_{0}}-\excconst\geq\negconst-\abigconst+1-(\abigconst+\excconst)\cdot\extcovconst-\excconst\geq\abigconst-\abigconst+1=1$.
    The total effect on the counter $i'\in\concincount\setminus\set{i}$ from the left is at least $-\abigconst+1+\excconst+\abigconst-\excconst\geq 1$.
    Similarly, the total effect on the counter $j\in\concoutcount$ from on the right is at most $-1$.
    This implies that $\incconst\neq\omega$, which is a contradiction.
\end{proof}

As a corollary to the proof of \Cref{Lemma:GuaranteedContradictionSimple}, we observe that a similar statement holds if $\concincount=\concoutcount$.

\begin{corollary}\label{Corollary:GuaranteedContradictionFullConcRaw}
    Let $\booleanflagof{\domain}=\bot$.
    Let $\atree$ be a witness tree with root label $(\amarkingin, \anonterminalin, \amarkingp)$ and $\omegaof{\amarkingin}=\omegaincount$, let $\concoutcount\subset\concincount$, and let $\abigconst=\sum_{j\in\concincount}\cardof{\amarkingin[j]}+\sum_{j\in\concoutcount}\cardof{\amarkingp[j]}$.
    Further let $\atree$ contain a node labeled $(\amarking, \anonterm, \amarkingpp)$, where $\amarking[i],\amarkingpp[j]\geq\negconst$ for $\negconst=(\extcovconst+\abigconst+1)\cdot(\extcovconst+1)$, $i\in\concincount$, and $j\in\concoutcount$.
    Then, $(\amarking, \anonterm, \amarkingpp)\in\simplydecomps$.
\end{corollary}

Finally, we observe that the output values cannot be too small, if the input values are of a certain size.

\begin{lemma}\label{Lemma:BoundedDivergence}
    Let $\atree$ be a witness tree with root label $(\amarkingin, \anonterminalin, \amarkingp)$, and $\concincount=\concoutcount$.
    Then, if $(\amarking, \anonterm, \amarkingp)$ is the label of a node in $\atree$, and $\amarking[i]\geq 2\cdot\solthresholdof{\bigoof{d\cdot\abigconst}+\bigoof{d\cdot \abigconst'}+\cardof{\chareq{\anngvas}}}+1$ for some $\abigconst\in\N$, where $\abigconst'=\sum_{j\in\concincount}\cardof{\amarkingin[j]}+\sum_{j\in\concoutcount}\cardof{\amarkingp[j]}$ and $i\in\concincount$, then there is a $j\in\concincount$ such that $\amarkingpp[j]\geq\abigconst$.
\end{lemma}

\begin{proof}
    Let $\atree$ be a witness tree, and $(\amarking, \anonterm, \amarkingpp)$ be as stated in the lemma.
    Suppose that for all $j\in\concincount$, $\amarkingpp[j]\leq\abigconst$.
    By a similar argument to \Cref{Lemma:OneSideGuaranteesPump}, we observe that there must be a solution $\asol_{\anonterm}$ to $\otherctxNGVAS{\anngvas}{\amarking, \anonterm, \outof{\anonterm}}$ with input values $\amarking$ and output values $\amarkingp+c_{\mathsf{hom}}$, where $c_{\mathsf{hom}}\in\N^{d}$ with $c_{\mathsf{hom}}[i]\geq \solthresholdof{\bigoof{d\cdot\abigconst'}+\cardof{\chareq{\anngvas}}}+1$.
    The witness tree $\atree$ corresponds to a solution $\asol$.
    Substracting the Parikh vector that coresponds to the subtree below $(\amarking, \anonterm, \amarkingpp)$, and adding $\asol_{\anonterm}$ gives us a new solution to $\otherctxNGVAS{\anngvas}{\amarkingin, \anonterminalin, \outof{\anonterminalin}}$, where the input value is a specialization of $\amarkingin$, but the output value is a specialization of $\amarkingp+c$, where $\omegaof{\amarkingp}=\omegaoutcount=\omegaincount$.
    Since the equation system for $\otherctxNGVAS{\anngvas}{\amarking, \anonterminalin, \outof{\anonterminalin}}$ has size at most $\bigoof{d\cdot \abigconst'}+\cardof{\chareq{\anngvas}}$, it must hold that $\sum_{i'\in \concincount}\amarkingp[i'] + c[i']\leq \solthresholdof{\bigoof{d\cdot\abigconst'}+\cardof{\chareq{\anngvas}}}$.
    But, this contradicts $c[i]\geq \solthresholdof{\bigoof{d\cdot\abigconst'}+\cardof{\chareq{\anngvas}}}+1$.
\end{proof}

Combining \Cref{Corollary:GuaranteedContradictionFullConcRaw} and \Cref{Lemma:BoundedDivergence}, we get that \Cref{Lemma:UsefulRestriction} holds in the case $\booleanflagof{\domain}=\bot$.

\begin{corollary}\label{Corollary:UsefulRestrictionBotCase}
    Let $\booleanflagof{\domain}=\bot$, and let $\atree$ be a witness tree with root label $(\amarkingin, \anonterminalin, \amarkingp)$.
    We can compute a $\domainconst\in\N$, so that for all nodes with labels $(\amarking, \anonterm, \amarkingpp)$ where $\amarking[i]\geq\domainconst$ for some $i\in\concincount$, it must hold that $(\amarking, \anonterm, \amarkingpp)\in\simplydecomps$.
\end{corollary}

\subsection{Proof of \Cref{Proposition:Precalculation}}\label{Section:Precalculation}

Now, we show that \Cref{Proposition:Precalculation} holds.

\noindent\textit{Computing $\excconst$.}
Note that by our assumption on $\anngvas$, the base effects of all childNGVAS $\anngvasp$ correspond to some $\abaserunof{\anngvasp}\in\runsof{\anngvas}$.
We can effectively construct such a run, and we have $\sizeof{\abaserunof{\anngvasp}}=\sum_{\anupd\in\updates}\sizeof{\anupd}\cdot\anngvasp.\avec[i]$.
Then, for any $\asentform=\asentform[0]\ldots\asentform[k]\in\terms^{*}$, we let $\abaserunof{\asentform}=\abaserunof{\asentform[0]}\ldots\abaserunof{\asentform[k]}$.
Clearly, we can also construct $\abaserunof{\asentform}$, and we have $\abaserunof{\asentform}\in\runsof{\asentform}$.  
Note that, since $\anngvas$ is strongly connected, there is a derivation $\anonterm\to\asentform.\anontermp.\asentformp$ in the grammar of $\anngvas$ for any $\anonterm, \anontermp\in\nonterms$.
Now, we put everything together to compute $\excconst$.
For each $\anonterm, \anontermp\in\nonterms$, we let $\excconstof{\anonterm, \anontermp}=\max(\sizeof{\abaserunof{\asentform}}, \sizeof{\abaserunof{\asentformp}})$, where $\anonterm\to\asentform.\anontermp.\asentformp$.
We let $\excconst=\max_{\anonterm, \anontermp\in\nonterms}\excconstof{\anonterm, \anontermp}$.
As a consequence of our arguments, this can be computed, and fulfills the specification in \Cref{Proposition:Precalculation}.\\

\noindent\textit{Computing $\incconst$.}
In order to use it later when we compute $\extcovconst$ and $\extcovmap$, we compute a more general version of $\incconst$.
We claim that we can compute the following function.
\begin{lemma}
    For all $K, L\subseteq[1, d]$ we can compute the value $\incconstCof{\anonterm}{K, L}\in\Nomega$ where if $\incconstCof{\anonterm}{\Nomega}\in\N$, then there is a derivation $\anonterm\to\asentform.\anonterm.\asentformp$ with $\arun\in\runsof{\asentform}$, $\arunp\in\runsof{\asentformp}$, where $\cteffectof{\arun}[i]\geq 1$ and $-\cteffectof{\arunp}[j]\geq 1$ for any $i\in K$, $j\in L$.
    If $\incconstCof{\anonterm}{K, L}=\omega$, then there is no such derivation.
\end{lemma}
This already implies the relevant portion of \Cref{Proposition:Precalculation}.
Letting $\incconst=\max_{\anonterm\in\nonterms}\incconstCof{\anonterm}{\adimset\setminus\omegaincount, \adimset\setminus\omegaoutcount}$ shows the $\incconst$-related item in \Cref{Proposition:Precalculation}.

Towards constructing $\incconstCof{\anonterm}{K, L}$, we check whether there is a derivation $\anonterm\to\asentform.\anonterm.\asentformp$, and for each applicable $i$, and $\asentformpp\in\set{\asentform, \asentformpp}$, a vector  $\ahomsol_{i, \asentformpp}\in\asentformpp[i].\periodeffect^{*}$ with 
$$(\sum_{i<\cardof{\asentform}}\asentform[i].\baseeffect+\ahomsol_{i, \asentform})[a]\geq 1$$
for all $a\in K$, and 
$$-(\sum_{i<\cardof{\asentformp}}\asentformp[i].\baseeffect+\ahomsol_{i, \asentformp})[b]\geq 1$$
for all $b\in L$.
This check can be effectively done by e.g. the construction of a Parikh image.
If this derivation and sequence of vectors does not exist, it is clear that the $\Z$-pumping derivation cannot exist, and we let $\incconstCof{\anonterm}{K, L}=\omega$.
For all $c\in\N$, $a\in K$, and $b\in L$, we have 
$$(\sum_{i<\cardof{\asentform}}c\cdot\asentform[i].\baseeffect+c\cdot\ahomsol_{i, \asentform})[a]\geq c$$
and 
$$-(\sum_{i<\cardof{\asentformp}}c\cdot\asentformp[i].\baseeffect+c\cdot\ahomsol_{i, \asentformp})[b]\geq c.$$
Choose a large enough $c\in\N$ such that it is strictly larger than $\sum_{\aperiod\in\anngvasp.\periodeffect}\sizeof{\aperiod}$.
Now let $\ahomsol_{i, \asentformpp}'=c\cdot\ahomsol_{i, \asentformpp}+\sum_{\aperiod\in\asentformpp[i].\periodeffect}\aperiod$ for each $i<\asentformpp$.
For all $a\in K$, and $b\in L$ we have 
$$(\sum_{i<\cardof{\asentform}}c\cdot\asentform[i].\baseeffect+\ahomsol_{i, \asentform}')[a]\geq 1$$
and 
$$-(\sum_{i<\cardof{\asentformp}}c\cdot\asentformp[i].\baseeffect+\ahomsol_{i, \asentformp}')[b]\geq 1.$$
Observe that $\ahomsol_{i, \asentformpp}'$ is a full period vector that allows us to apply \Cref{TheoremIterationLemmaNonLinearOverview}.
We apply \Cref{TheoremIterationLemmaNonLinearOverview} to get $C$ larger than the $k_{0}$ of $\asentformpp[i]$ given by \Cref{TheoremIterationLemmaNonLinearOverview} for the full period vector $\ahomsol_{i, \asentformpp}'$, for all $\asentformpp\in\set{\asentform, \asentformp}$ and $i<\sizeof{\asentformpp}$.
Then, 
$$(\sum_{i<\cardof{\asentform}}C\cdot c\cdot\asentform[i].\baseeffect+C\cdot \ahomsol_{i, \asentform}')[a]\geq C$$
and 
$$-(\sum_{i<\cardof{\asentformp}}C\cdot c\cdot\asentformp[i].\baseeffect+C\cdot \ahomsol_{i, \asentformp}')[b]\geq -C.$$
Furthermore, for each $\asentformpp\in\set{\asentform, \asentformp}$ and $i<\cardof{\asentformpp}$, we construct the run $\apumpedrunof{\asentformpp[i]}{C}$, where $\apumpedrunof{\asentformpp[i]}{C}\in\runsof{\asentformpp[i]}$ is the run delivered by \Cref{TheoremIterationLemmaNonLinearOverview}.
We have $\paramparikhof{\updates}{\apumpedrunof{\asentformpp[i]}{C}}=C\cdot\ahomsol_{i, \asentform'}$.
Therefore, for all $a\in K$
$$(\sum_{i<\cardof{\asentform}}C\cdot c\cdot\asentform[i].\baseeffect+\cteffectof{\apumpedrunof{\asentform[i]}{C}})[a]\geq C$$
which implies 
$$(\sum_{i<\cardof{\asentform}}C\cdot c\cdot\cteffectof{\abaserunof{\asentform[i]}}+\cteffectof{\apumpedrunof{\asentform[i]}{C}})[a]\geq C$$
We similarly get 
$$(\sum_{i<\cardof{\asentformp}}C\cdot c\cdot\cteffectof{\abaserunof{\asentformp[i]}}+\cteffectof{\apumpedrunof{\asentformp[i]}{C}})[b]\geq C.$$
for all $b\in L$.
We know that 
$$\apumpedrunof{\asentformpp}{C}:=\apumpedrunof{\asentformpp[0]}{C}\ldots\apumpedrunof{\asentformpp[\cardof{\asentformpp}-1]}{C}\in\runsof{\asentformpp}$$
and 
$$\abaserunof{\asentformpp}=\abaserunof{\asentformpp[0]}\ldots\abaserunof{\asentformpp[\cardof{\asentformpp}-1]}\in\runsof{\asentformpp}$$
for all $\asentformpp\in\set{\asentform, \asentformp}$.
We let
$$\arun_{\asentformpp}^{\incconst}:=\apumpedrunof{\asentformpp}{C}.(\abaserunof{\asentformpp})^{C\cdot c-1}\in\runsof{\asentformpp^{C\cdot c}}$$
for $\asentformpp\in\set{\asentform, \asentformp}$.
By our previous arguments, 
$$\cteffectof{\arun_{\asentform}^{\incconst}}[a]\geq 1\qquad \cteffectof{\arun_{\asentformp}^{\incconst}}[b]\geq 1$$
for all $a\in K$, and $b\in L$.
Since we also have $\anonterm\to\asentform^{C\cdot c}.\anonterm.\asentformp^{C\cdot c}$, $\arun_{\asentform}^{\incconst}\in\runsof{\asentform^{C\cdot c}}$, and $\arun_{\asentformp}^{\incconst}\in\runsof{\asentformp^{C\cdot c}}$, we let $\incconstCof{\anonterm}{K, L}=\max(\sizeof{\arun_{\asentform}^{\incconst}}, \sizeof{\arun_{\asentformp}^{\incconst}})$ and conclude the proof.\\

\noindent\textit{Computing $\extcovmap$ and $\extcovconst$.}
We compute $\extcovmap$ and $\extcovconst$ simultaneously.
As a preliminary, we observe
\begin{lemma}\label{Lemma:PumpingLength}
    Let $\amarking, \amarkingp\in\Nomega$ and $\anonterm\in\nonterms$ with $\omegaof{\amarking}, \omegaof{\amarkingp}\supsetneq\omegaincount$, $\amarking\sqsubseteq\inof{\anonterm}$, $\amarkingp\sqsubseteq\outof{\anonterm}$.
    We can compute $\pumpinglengthof{\amarking, \anonterm, \amarkingp}\in\Nomega$, where $\pumpinglengthof{\amarking, \anonterm, \amarkingp}=\omega$, if $(\amarking, \anonterm, \amarkingp)$ does not admit a pumping derivation, and if $\pumpinglengthof{\amarking, \anonterm, \amarkingp}\in\N$, then $(\amarking, \anonterm, \amarkingp)$ admits a pumping derivation $\anonterm\to\asentform.\anonterm.\asentformp\in\terms^{*}.\anonterm.\terms^{*}$, and $\arun_{\mathsf{pump}}\in\runsof{\asentform}$, $\arunp_{\mathsf{pump}}\in\runsof{\asentformp}$ with $\pumpinglengthof{\amarking, \anonterm, \amarkingp}\geq\max(\sizeof{\arun}, \sizeof{\arunp})$.
\end{lemma}

\begin{proof}
    Computability of $\pumpinglengthof{\amarking, \anonterm, \amarkingp}=\omega$ amounts to checking \perfectnesspumping for $\otherctxNGVAS{\anngvas}{\amarking, \anonterm, \amarkingp}$ which can be done by \Cref{Lemma:WitnessGrammarTermination} and \Cref{Lemma:EasilyComputableCG} for $\amarking$, $\amarkingp$ as given in the lemma.
    If $\pumpinglengthof{\amarking, \anonterm, \amarkingp}\neq\omega$, we enumerate all derivations until we find a pumping derivation. 
\end{proof}

The challenge in computing $\extcovmap$ and $\extcovconst$ is capturing the upward closure of \emph{all} possible pumping derivations.
In order to do this, we use $\incconstCof{\anonterm}{K, L}$ for help.
Once we have $\extcovmap$ at hand, computing $\extcovconst$ is trivial with the help of \Cref{Lemma:PumpingLength}.
In order to construct $\extcovmap$, we define a recursive procedure $\pumpingconstruct{\anincount, \anoutcount}:\Nomega^{d}\times\nonterms\times\Nomega^{d}\to\powof{\Nomega^{d}\times\nonterms\times\Nomega^{d}}$, that fulfills the following specification.
\begin{lemma}\label{Lemma:ConstructingExtCovMap}
    Let $\anincount, \anoutcount\subsetneq\concincount$, and $\anoutcount\subseteq\concoutcount$.
    We can compute $\pumpingconstruct{\anincount, \anoutcount}:\Nomega^{d}\times\nonterms\times\Nomega^{d}\to\powof{\Nomega^{d}\times\nonterms\times\Nomega^{d}}$.
    Then, for all labelings $(\amarking, \anonterm, \amarkingp)\in\Nomega^{d}\times\nonterms\times\Nomega^{d}$ with $\omegaof{\amarking}=[1,d]\setminus\anincount$, and $\omegaof{\amarkingp}=[1,d]\setminus\anoutcount$, we have $(\amarking, \anonterm, \amarkingp)\in\upclsof{\pumpingconstructof{\anincount, \anoutcount}{\inof{\anonterm}, \anonterm, \outof{\anonterm}}}$ if and only if $(\amarking, \anonterm, \amarkingp)$ admits a pumping derivation.
\end{lemma}

\Cref{Lemma:ConstructingExtCovMap} readily implies the $\extcovmap$ portion of \Cref{Proposition:WitnessGrammarDecomp}.
We can simply let 
$$\extcovmap=\bigcup_{\anincount\subsetneq\concincount}\;\bigcup_{\anoutcount\subseteq\concoutcount, \anoutcount\subsetneq\concincount}\;\bigcup_{\anonterm\in\nonterms}\pumpingconstructof{\anincount, \anoutcount}{\inof{\anonterm}, \anonterm, \outof{\anonterm}}.$$

Let $\anincount, \anoutcount\subsetneq\concincount$, and $\anoutcount\subseteq\concoutcount$.
We present $\pumpingconstructof{\anincount}{\amarking, \anonterm, \amarkingp}$ for label $(\amarking, \anonterm, \amarkingp)\in\Nomega^{d}\times\nonterms\times\Nomega^{d}$ below.
For a vector $\amarking$, we let $\amarking_{\softsetter{K}{v}}$ agree with the vector $\amarking$ on concrete positions and on positions outside of $K\subseteq [1,d]$, and has $v\in\N$ on the remaining positions. 
\begin{align*}
    \intertext{Define $k=\incconstCof{\anonterm}{\anincount\cap\adimset, \anoutcount\cap\adimset}\cdot(\pumpinglengthof{\amarking, \anonterm, \amarkingp}+ 1)$.}
    \pumpingconstructof{\anincount, \anoutcount}{\amarking, \anonterm, \amarkingp}&=
    (\amarking_{\softsetter{\anincount}{k}}, \anonterm, \amarking_{\softsetter{\anoutcount}{k}})\\
    &\cup\bigcup_{i\in\anincount\cap\omegaof{\amarking}}\bigcup\setcond{\pumpingconstructof{\anincount, \anoutcount}{\amarking_{\softsetter{i}{l}}, \anonterm, \amarkingp}}{\\
    &\hspace{6.5em}l<k,\; \pumpinglengthof{\amarking_{\softsetter{i}{l}}, \anonterm, \amarkingp}\neq\omega}\\
    &\cup\bigcup_{i\in\anoutcount\cap\omegaof{\amarkingp}}\bigcup\setcond{\pumpingconstructof{\anincount, \anoutcount}{\amarking, \anonterm, \amarkingp_{\softsetter{i}{l}}}}{\\
    &\hspace{6.5em}l<k,\; \pumpinglengthof{\amarking, \anonterm, \amarkingp_{\softsetter{i}{l}}}\neq\omega}
\end{align*}
The procedure $\pumpingconstructof{\anincount, \anoutcount}{\amarking, \anonterm, \amarkingp}$ expects the input with $\anincount\cup\omegaof{\amarking}=\anoutcount\cup\omegaof{\amarkingp}=\omega$.
Then, it constructs $k$ using $\incconstof{\anonterm}$ and $\pumpinglengthof{\amarking, \anonterm, \amarkingp}$.
Because of the choice of $\anincount$ and $\anoutcount$, \Cref{Lemma:PumpingLength} implies that it is computable.
By a similar argument to \Cref{Lemma:GuaranteedPump}, we know that $(\amarking_{\softsetter{\anincount}{k}}, \anonterm, \amarking_{\softsetter{\anoutcount}{k}})$ must admit a pumping derivation.
The procedure than concretizes one counter $i\in\anincount$ or $j\in\anoutcount$ with a value less than $k$ and calls $\pumpingconstruct{\anincount, \anoutcount}$ again.
Here, it makes sure that that the concretization still admits a pumping derivation.
We argue termination via the number of $\omega$'s in the input.
If all counters from $\anincount$ in the input, and from $\anoutcount$ in the output are concrete, then the function returns the input value.
If not, then all the following calls have one more concrete counter than the input.

We argue that $\pumpingconstruct{\anincount, \anoutcount}$ fulfills \Cref{Lemma:ConstructingExtCovMap}.
We argue by induction on the number of $\omega$'s that if $(\amarking', \anonterm, \amarkingp')$ admits a pumping derivation, has the concrete counters $\anincount$, $\anoutcount$, and is a specialization of $(\amarking, \anonterm, \amarkingp)$, then it is captured in $\upclsof{\pumpingconstructof{\anincount, \anoutcount}{\amarking, \anonterm, \amarkingp}}$.
Since all labelings $(\amarking, \anonterm, \amarkingp)$ are specializations of $(\inof{\anonterm}, \anonterm, \outof{\anonterm})$, the result follows.
The argument for the inductive step is the following. 
Let $(\amarking', \anonterm, \amarkingp')$ not be contained in $(\amarking_{\softsetter{\anincount}{k}}, \anonterm, \amarking_{\softsetter{\anoutcount}{k}})$.
If it is, then we are done. 
Then, one counter $i\in\anincount$ or $j\in\anoutcount$ must be $\omega$ on the corresponding side of $(\amarking, \anonterm, \amarkingp)$, but less than $k$ in $(\amarking', \anonterm, \amarkingp')$. 
By the induction hypothesis, this must be captured in one of the subcalls. 
This concludes the proof.
